# Supplementary material for: Neural-Enhanced Dynamic Range Compression Inversion: A Hybrid Approach for Restoring Audio Dynamics
Source: arXiv:2411.04337 source file (2025-09-09)
Supplement: Supplementary file 1 [file appendix.tex]

% {\appendix[Proof of the Zonklar Equations]
% Use $\backslash${\tt{appendix}} if you have a single appendix:
% Do not use $\backslash${\tt{section}} anymore after $\backslash${\tt{appendix}}, only $\backslash${\tt{section*}}.
% If you have multiple appendixes use $\backslash${\tt{appendices}} then use $\backslash${\tt{section}} to start each appendix.
% You must declare a $\backslash${\tt{section}} before using any $\backslash${\tt{subsection}} or using $\backslash${\tt{label}} ($\backslash${\tt{appendices}} by itself
%  starts a section numbered zero.)}

{\appendices
\section{Detail of the 30 DRC profiles}
\label{sec:30profiles}

The following table shows the detailed parameters of the 30 DRC profiles used for generating the large compressed signal datasets. The detector type of all the profiles is set to 2, which corresponds to the RMS detector.

\begin{table}[!ht]
\centering
\caption{Detailed parameters of the used 30 DRC profiles.}

\resizebox{\linewidth}{!}{
\begin{tabular}{c|c|c|c|c|c|c}
\toprule
Profile & L & R & $\tau_v^{att}$ & $\tau_v^{rel}$ & $\tau_g^{att}$ & $\tau_g^{rel}$ \\ \hline
1 & -30.6 & 2.3 & 73.9 & 20.3 & 451.5 & 1153.6 \\
2 & -55.9 & 12.1 & 25.4 & 50.9 & 54.1 & 1274.5 \\
3 & -55.1 & 13.4 & 43.3 & 76.4 & 354.6 & 468.4 \\
4 & -39.6 & 13.1& 66.2 & 10.1 & 325.5 & 1435.7 \\
5 & -31.4 & 12.3 & 99.4 & 91.7 & 160.7 & 790.8 \\
6 & -60.0 & 15.0 & 130.0 & 89.2 & 393.4 & 1758.2 \\
7 & -47.8 & 5.4 & 50.9 & 84.1 & 403.1 & 1677.6 \\
8 & -46.9 & 4.9 & 48.4 & 66.2 & 257.7 & 1516.3 \\
9 & -45.3 & 2.5 & 89.2 & 114.7 & 344.9 & 1234.2 \\
10 & -26.5 & 10.8 & 114.7 & 68.8 & 209.2 & 145.9 \\
11 & -43.7 & 8.4 & 35.6 & 107.0 & 432.1 & 750.5 \\
12 & -20.8 & 6.5 & 84.1 & 101.9 & 500.0 & 347.4 \\
13 & -22.4 & 11.3 & 124.9 & 63.7 & 364.3 & 831.1 \\
14 & -40.4 & 10.0 & 112.1 & 99.4 & 374.0 & 1355.1 \\
15 & -52.7 & 4.4 & 104.5 & 35.6 & 199.5 & 1919.4 \\
16 & -51.8 & 2.0 & 117.2 & 117.2 & 277.0 & 549.0 \\
17 & -38.0 & 5.2 & 5.0 & 40.7 & 296.4 & 1717.9 \\
18 & -51.0 & 3.3 & 28.0 & 127.4 & 170.4 & 669.9 \\
19 & -29.8 & 9.2 & 33.1 & 56.0& 131.6 & 1959.7 \\
20 & -29.0 & 11.8 & 45.8 & 81.5 & 412.8 & 992.3 \\
21 & -28.2 & 5.7 & 10.1 & 17.8 & 34.7 & 428.1 \\
22 & -50.2 & 12.6 & 22.9 & 122.3 & 83.2 & 1395.4 \\
23 & -23.3 & 12.9 & 12.7 & 7.6 & 112.2 & 25.0 \\
24 & -44.5 & 7.8 & 15.2 & 86.6 & 306.1 & 1838.8 \\
25 & -46.1 & 11.0 & 122.3 & 12.7 & 189.8 & 1113.3 \\
26 & -56.7 & 2.8 & 94.3 & 28.0 & 102.6 & 186.2\\
27 & -24.9 & 10.5 & 38.2 & 43.3 & 335.2 & 226.5 \\
28 & -48.6 & 8.9& 107.0 & 104.5 & 25.0 & 1798.5 \\
29 & -49.4 & 10.2 & 127.4 & 71.3 & 92.9 & 508.7 \\
30 & -24.1 & 14.2 & 81.5 & 58.6 & 180.1 & 871.4 \\
\bottomrule
\end{tabular}}
\label{tab:30_drc_profiles}
\end{table}

\section{The detailed exploration of experimental results of using MFCC, MelS, and CQT as input features.}
\label{app:matrix}

The figures below show the detailed exploration of using the rest 3 $\text{TFR}_y$ as an input feature to the \ac{ast} model.
\begin{figure}[!ht]
  \centering
  \subfloat[Results for small datasets.]{\includegraphics[width=0.5\linewidth]{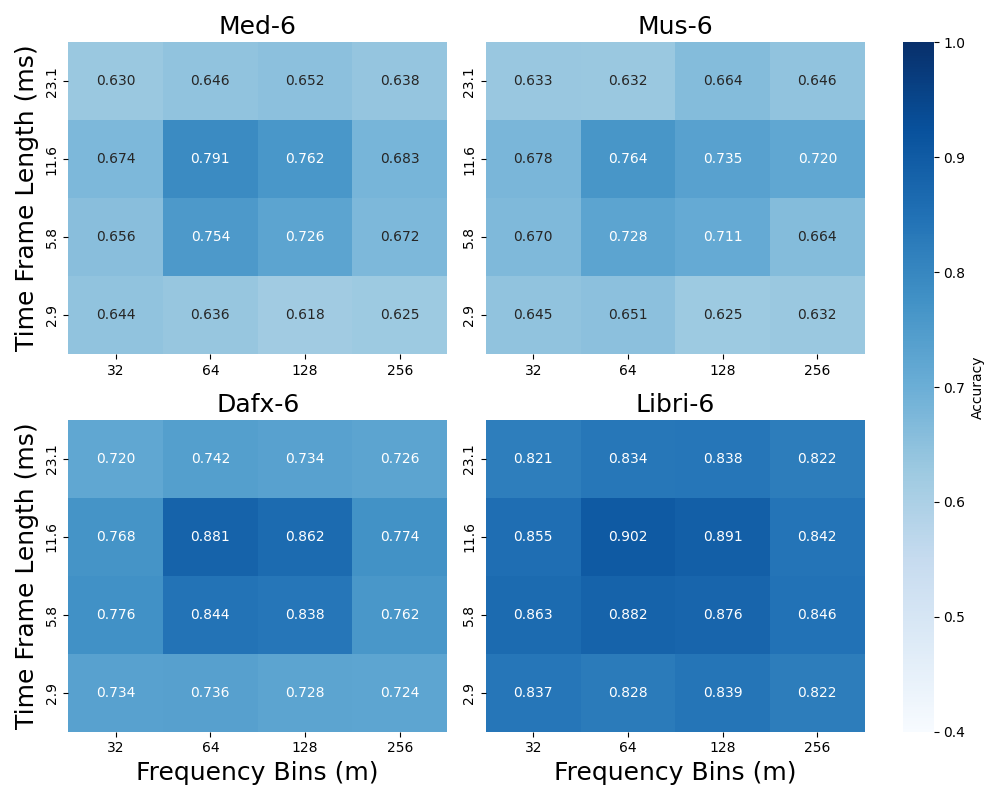}}
  \subfloat[Results for large datasets.]{\includegraphics[width=0.5\linewidth]{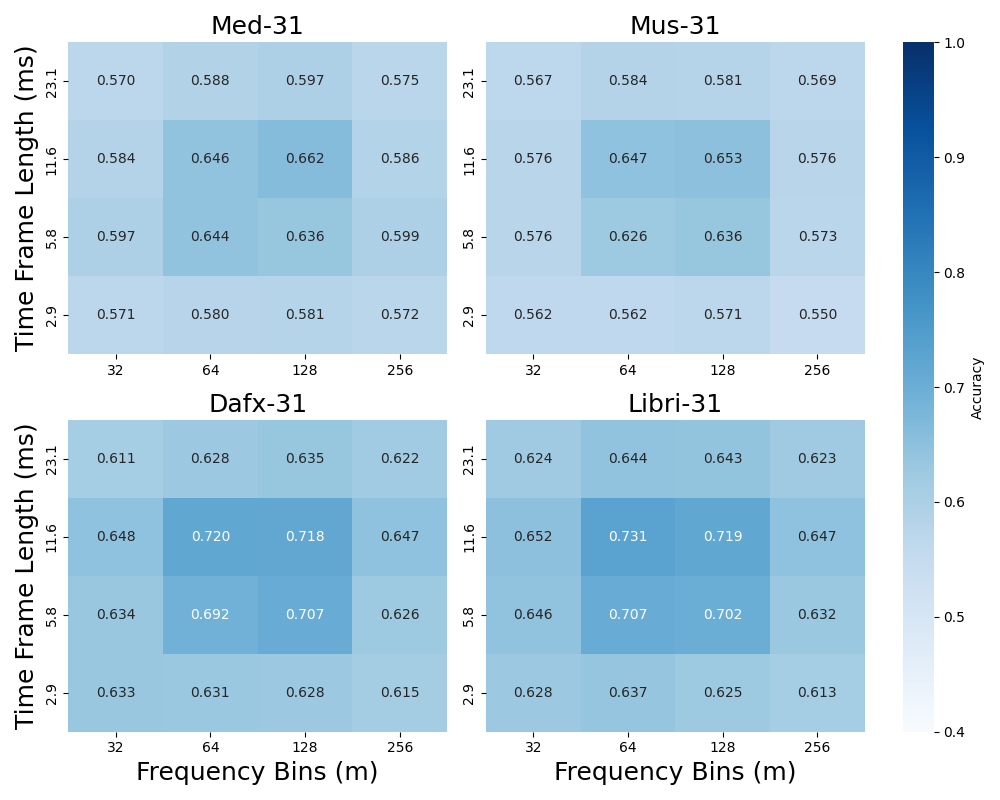}} \\
  \subfloat[Results for small datasets.]{\includegraphics[width=0.5\linewidth]{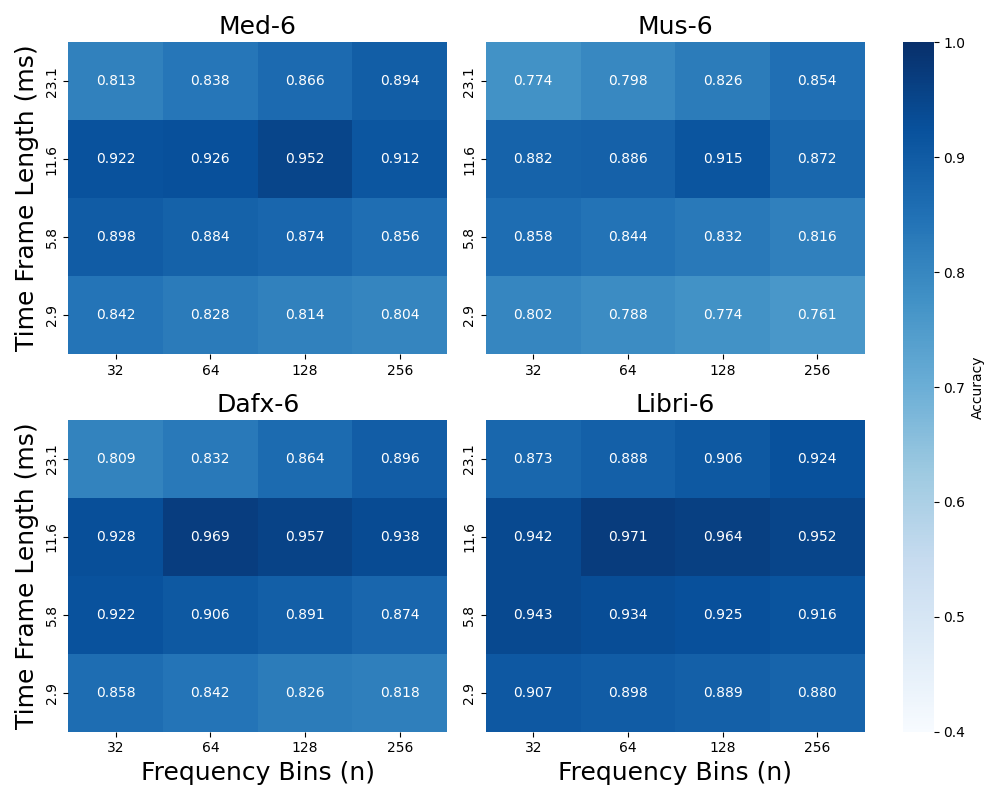}}
  \subfloat[Results for large datasets.]{\includegraphics[width=0.5\linewidth]{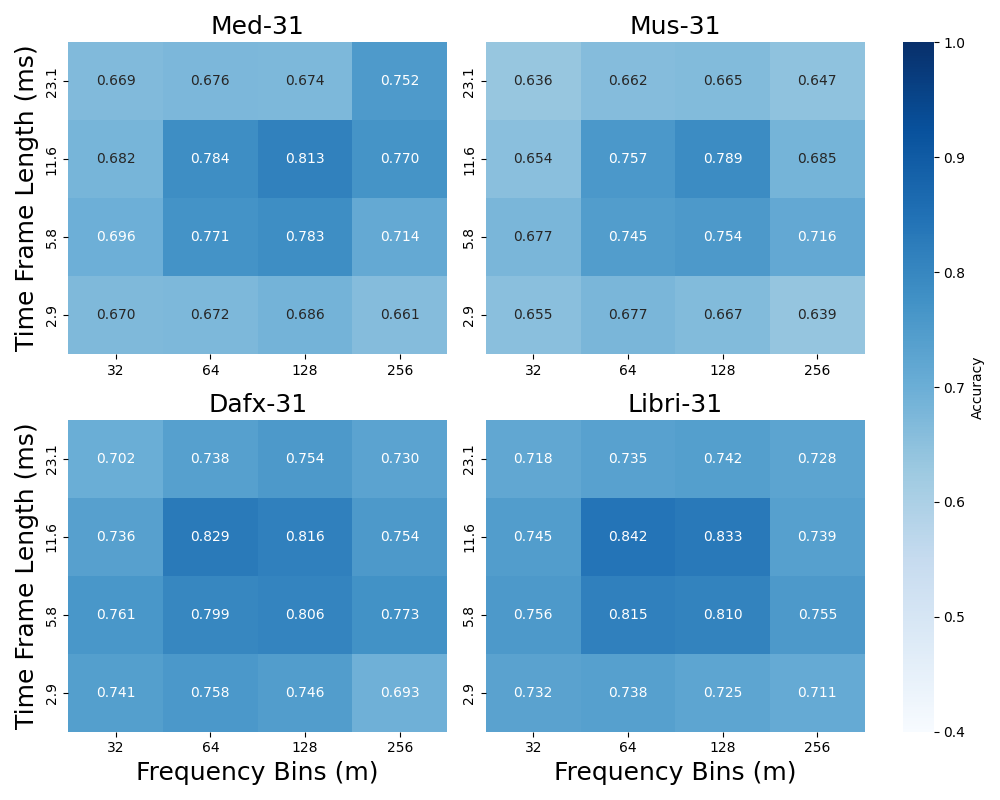}} \\
  \subfloat[Results for small datasets.]{\includegraphics[width=0.5\linewidth]{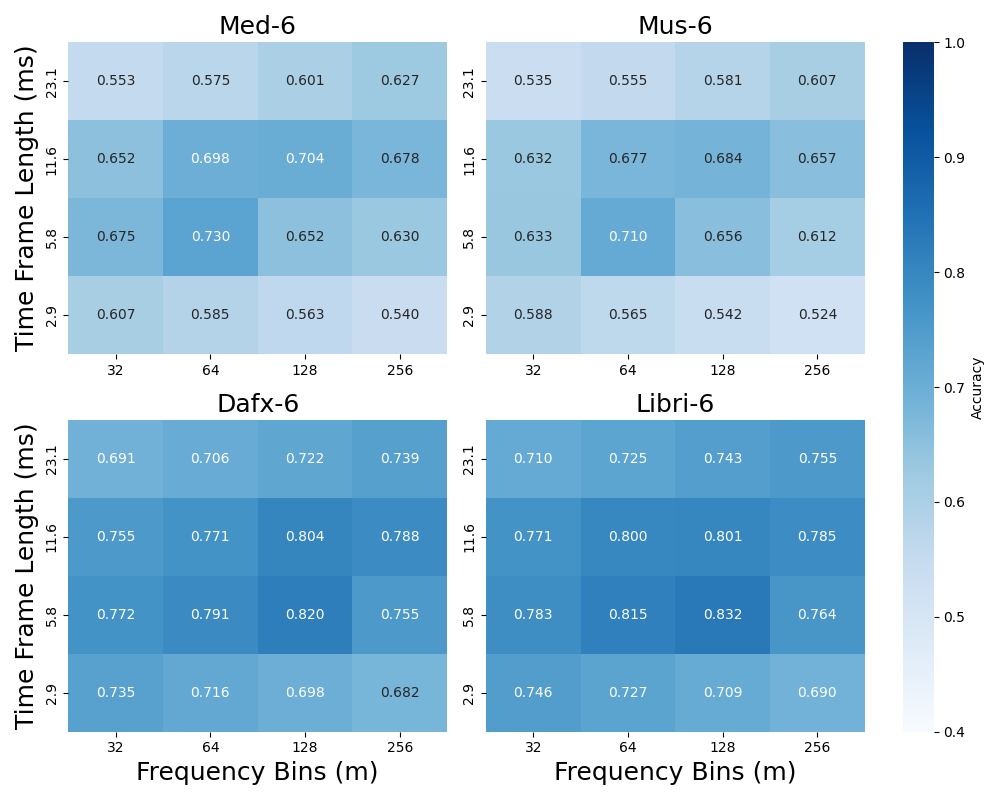}}
  \subfloat[Results for large datasets.]{\includegraphics[width=0.5\linewidth]{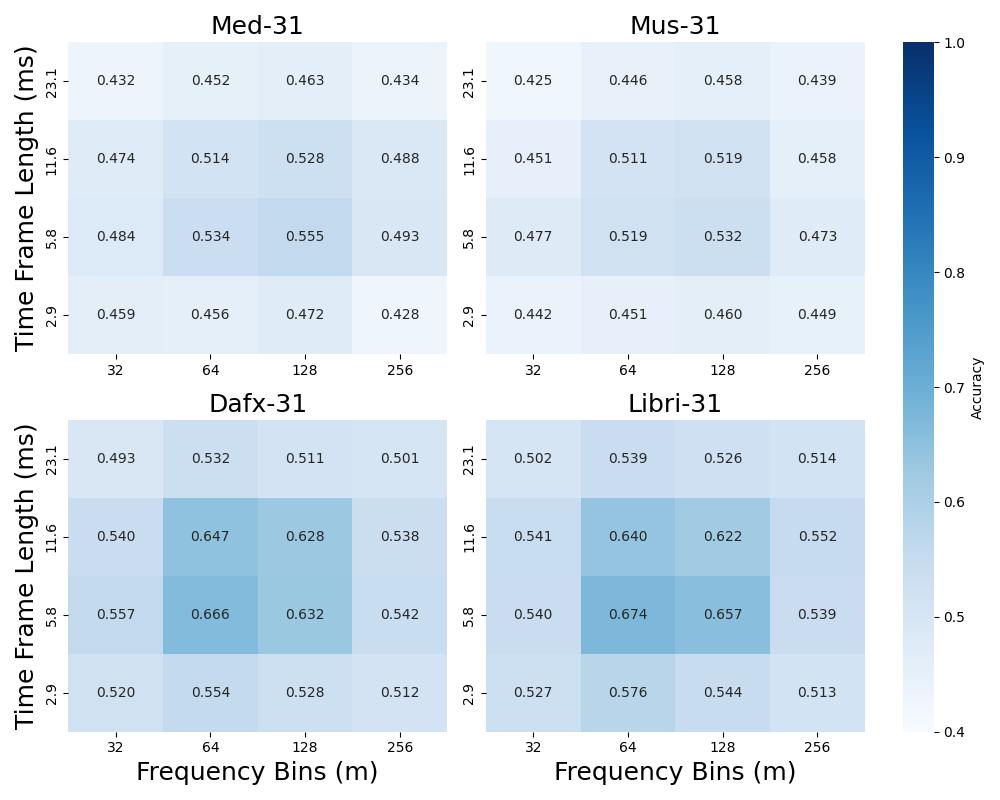}}
  \caption{Classification accuracy heatmaps about the impact of the size of the different $\text{TFR}_y$ on DRC profile classification using the \ac{ast} model.
  Figures (a) and (b) correspond to the results using MFCC; Figure (c) and (d) correspond to the results using MelS; Figure (e) and (f) correspond to the results using CQT.
  %The experiment investigates two scenarios: classification of 6 DRC profiles (top) and 31 DRC profiles (bottom). Each scenario tests four different datasets (Med, Mus, Dafx, and Libri). The x-axis represents the number of frequency bins (m), and the y-axis shows the time frame length (ms) used in the MFCC computation.
  }
  \label{fig:mat_3features}
\end{figure}
}

\section{References Section}
